# Supplementary material for: LLMs Lean on Priors, Not Programming Language Semantics
Source: arXiv:2510.03415 source file (2026-05-29)
Supplement: Supplementary file 1 [file notation_comprehension_dist.tex]

\begin{figure*}[h]%
  \centering%
  \subcaptionbox{\FigNotationComprehensionStdSosCaption}{%
    \resizebox{0.9\linewidth}{!}{%}
      \includegraphics{figures/appendix/nl2rule_uk.pdf}%
    }%
  }%
  \\
  \subcaptionbox{\FigNotationComprehensionNStdSosCaption}{%
    \resizebox{0.9\linewidth}{!}{%}
      \includegraphics{figures/appendix/nl2rule_mk.pdf}%
    }%
  }
  \\
  \subcaptionbox{\FigNotationComprehensionStdKCaption}{%
    \resizebox{0.9\linewidth}{!}{%}
      \includegraphics{figures/appendix/nl2rule_uk_k.pdf}%
    }%
  }
  \\
  \subcaptionbox{\FigNotationComprehensionNStdKCaption}{%
    \resizebox{0.9\linewidth}{!}{%}
      \includegraphics{figures/appendix/nl2rule_mk_k.pdf}%
    }%
  }
  \caption{\FigNotationComprehensionCaption}%
\end{figure*}%
