# Supplementary material for: LLMs Lean on Priors, Not Programming Language Semantics
Source: arXiv:2510.03415 source file (2026-05-29)
Supplement: Supplementary file 2 [file srp_most_correct_rules.tex]

\begin{figure}
  \hspace{2cm}\includegraphics[scale=0.28]{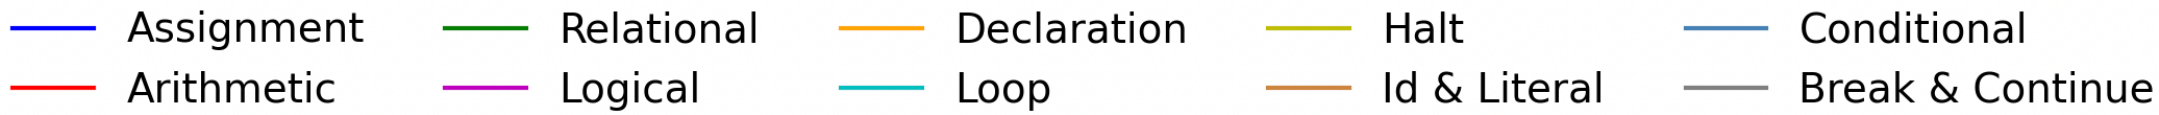}
  \vspace{2mm}
  \\
  \subcaptionbox{%
    \FigSRPUKRadarCaption%
    \label{figure:srp-uk-most-correct}}[0.3\linewidth]{%
    \includegraphics[scale=0.18]{figures/tasks/srp-uk-none-most-correct-rules-radar-chart.pdf}
  }%
  \hspace{5mm}%
  \subcaptionbox{%
    \FigSRPMKSwapRadarCaption%
    \label{figure:srp-mk-swap-most-correct}}[0.3\linewidth]{%
    \includegraphics[scale=0.18]{figures/tasks/srp-mk-replace-most-correct-rules-radar-chart.pdf}
  }%
  \hspace{5mm}%
  \subcaptionbox{%
    \FigSRPMKObfRadarCaption%
    \label{figure:srp-mk-obf-most-correct}}[0.3\linewidth]{%
    \includegraphics[scale=0.18]{figures/tasks/srp-mk-unseen-most-correct-rules-radar-chart.pdf}
  }%
  \caption{\FigSRPRadarMostCorrectRulesCaption}
\end{figure}
